# Supplementary material for: Effectively Prefetching Remote Memory with Leap
Source: arXiv:1911.09829 source file (2019-11-22)
Supplement: Supplementary file 1 [file appendix.tex]

\appendix

\section{Block Device I/O operation}
\label{app:bio-op}

\begin{figure}[!t]
  \centering
  \includegraphics[width=\columnwidth]{figures/2_io_operation}
  \caption{Basic flow diagram of I/O operations}
  \label{fig:io_operation}
\end{figure}

\todo{FIX.}

Any Direct Memory Access (DMA) operation inside the OS, must belong to adjacent sectors on disk. Each DMA setter-getter operation needs to have information about the disk storage area, address of the initial sector on disk and the number of sectors included in the operation. A block layer maintains the bio data structure to store the metadata of an I/O operation. 

At the beginning of a disk I/O operation, the OS allocates a bio descriptor for  the page and gathers information of all the sectors within the page. After checking the validity of the bio (\ie proper address space, access rights \etc), an I/O access request is generated, but, not initiated promptly. Rather, it is just scheduled into the request queue dedicated for that block device and the  process goes for a sleep. The block device intentionally delays the requests in a hope of gaining performance benefit. During the wait time, the tries to merge requests inside the queue to have more contiguous sectors in a single request. As large sequential disk access is always beneficial, the block layer tries to hide the disk seek time by deferred I/O operations. Eventually, the requests are asynchronously executed and the process is waken up when the I/O ends. Figure \ref{fig:io_operation} describes the basic flow of I/O operation in the presence of block device.
